# Supplementary material for: Ab initio study on lattice thermal conductivity of Cu$_2$O using GGA and hybrid density functional methods
Source: arXiv:1707.00434 source file (2017-07-03)
Supplement: Supplementary file 1 [file Supplemental_Material.pdf]

# Supplemental Material for "Ab initio study on lattice thermal conductivity of $Cu_2O$ using GGA and hybrid density functional methods"

J. Linnera and A. J. Karttunen

# I. BAND STRUCTURE CALCULATIONS AND ELECTRON DENSITIES

Figure 1 contains the band structures that were obtained using all combinations of functionals PBE, PBE0, and HSE06 with basis sets SVP, TZVP, and TZVPP. Shapes of the bands are very much alike with all functionals and differences between basis sets are barely visible. Band gaps with the TZVP basis set are 0.53 eV, 2.39, and 1.87 eV for PBE, PBE0, HSE06, respectively. The largest band gap difference between basis sets is seen with PBE0, where SVP produces 0.15 eV larger gap of 2.54 eV.

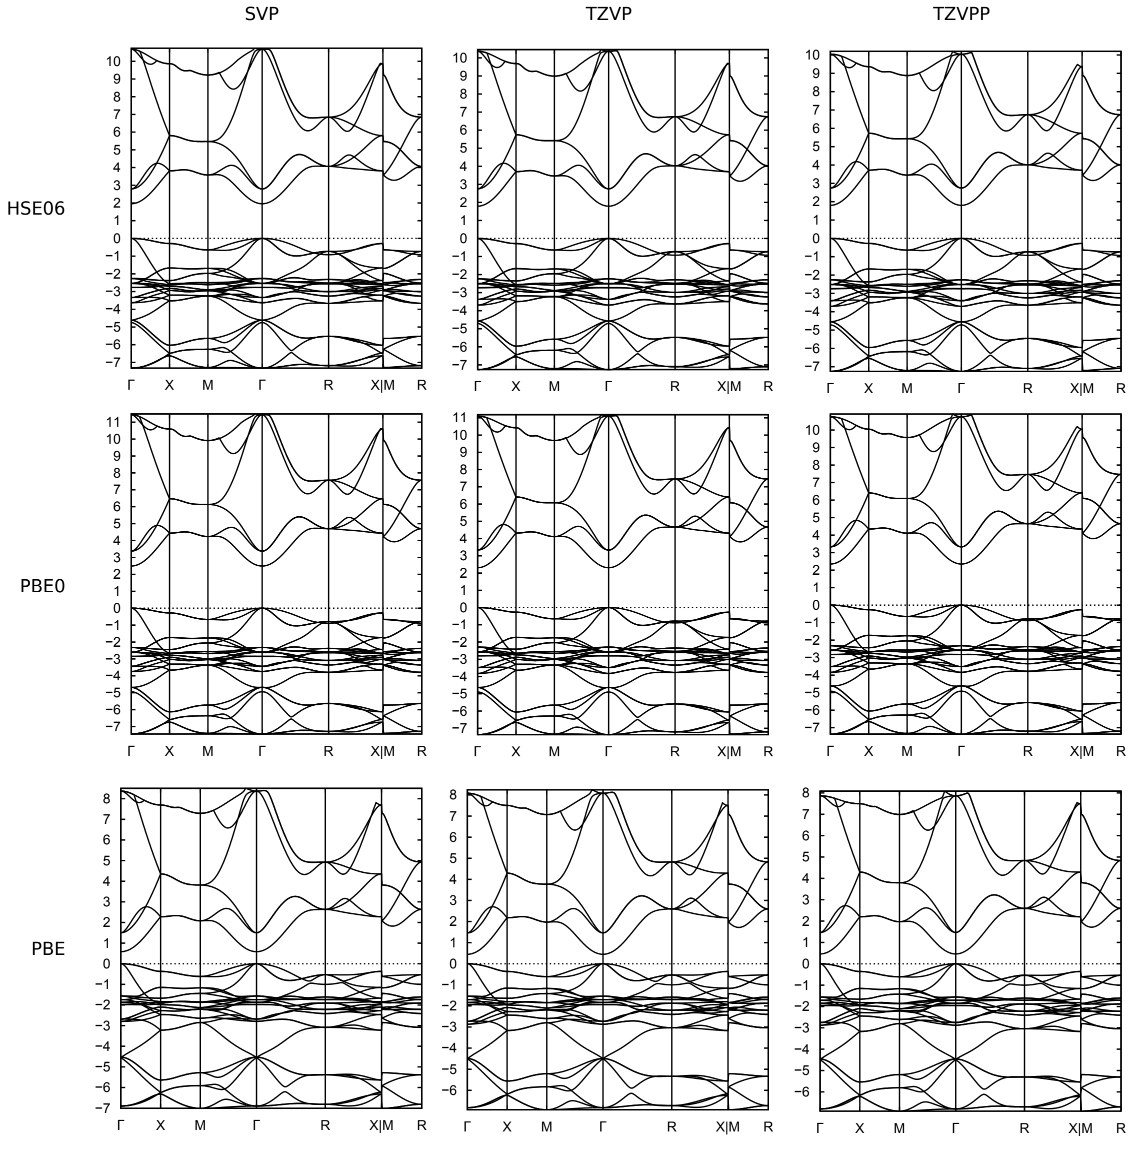


Figure 1. Band structures obtained with nine different functional/basis set combinations. Top of the valence bands is set to zero and marked with a dashed line.

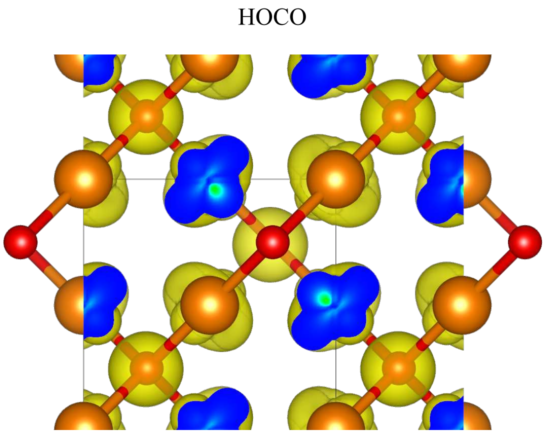


Figure 2. Band-projected electron densities for HOCO and HOCO-9 at the PBE0/TZVP level of theory (isovalue 0.005 a.u.). Red: O; brown: Cu; yellow: electron density; blue: cross-sections of the electron density

We also plotted the band-projected electron densities of the highest occupied crystalline orbital (HOCO) and HOCO-9 at the PBE0/TZVP level of theory (Figure 2). The density plots show the larger contribution from the oxygen $p$-states in the HOCO compared to HOCO-9. The latter comprises almost exclusively of copper $d$-states. The energy of the HOCO-9 band ranges from -2.75 eV to -2.57 eV below the valence band maximum.

## II. META-GGA PERFORMANCE

All calculations with the mGGAs were done using the TZVP basis set. Starting with the lattice parameters, the M06-L pure mGGA predicts $a$ = 4.308 Åand the hybrid M06 predicts $a$ = 4.327 Å. A similar overestimation of the lattice parameter is seen as with the other functionals tested in this study. While the GGA functional PBE produces a band gap of 0.53 eV, M06-L results in 0.58 eV. Similarly, hybrid functional PBE0 predicts a gap of 2.39 eV and the mGGA counterpart M06 a gap of 2.35 eV. A closer look on the band structure with M06 can be seen in Figure 3. Band structure is very similar to that of PBE0, and only slight differences can be seen in the DOS, mainly on the magnitudes. The amount of hybridization of O states in the valence bands is similar with both hybrid functionals PBE0 and M06.

We also calculated the full phonon dispersion using the hybrid M06 functional. As can be seen in Figure 4, the performance is very similar to PBE0. Some frequencies are found at

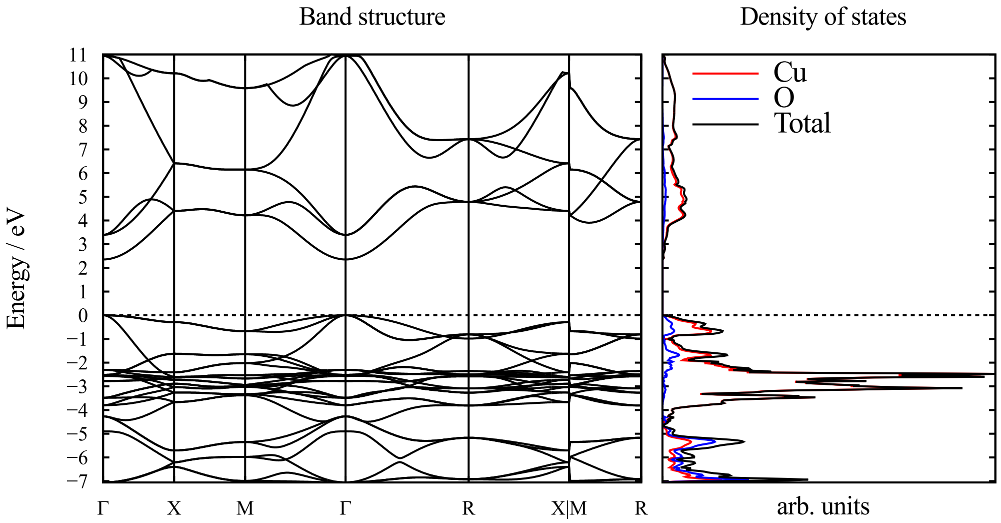


Figure 3. Band structure of $Cu_2O$ obtained with M06/TZVP level of theory.

smaller wavenumbers, e.g. in the Γ-point around 100 $cm^{-1}$, where PBE0 matches the experimental points near perfectly, while M06 does not. It should be noted that LO-TO splitting is not taken into account for M06 because the CPHF method for calculating the dielectric constants is not implemented in CRYSTAL for mGGA-functionals. Due to the similarity of PBE0 and M06 results and the technical limitations related to mGGA functionals in CRYSTAL, we did not pursue mGGA functionals further to calculate the third-order force constants with them. It should be noted that the recently developed semilocal SCAN mGGA functional[1] could improve the mGGA results at least in comparison to the non-hybrid M06-L functional.

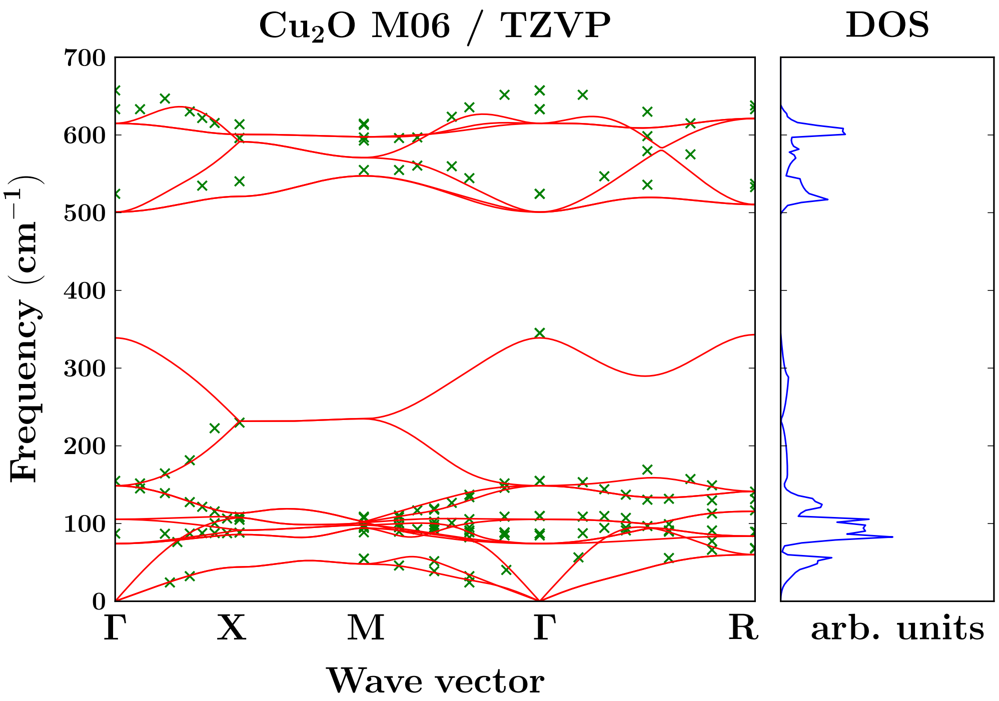


Figure 4. Phonon dispersion and PDOS of $Cu_2O$ obtained at the M06/TZVP level of theory. Red lines are our theoretical results, green crosses mark experimental data points from Ref[2]. The nonanalytical contribution when $\mathbf{q} \to 0$ is not taken into account.

## III. COMPARISON TO PLANE-WAVE BASIS

To confirm that the localized GTO-type basis set provides accurate force constants, we also calculated second-order force constants of $Cu_2O$ with Quantum ESPRESSO (QE) plane-wave code[3] both analytically (density-functional perturbation theory, DFPT[4]) and numerically (finite differences with Phonopy). We applied PBE functional and GBRV ultrasoft pseudopotentials with kinetic energy cut-offs of 40 Ry and 200 Ry for wavefunctions and charge densities, respectively.[5] We applied the same k-point meshes as in the CRYSTAL calculations and tight convergence criteria for the structural optimizations ($10^{-6}$ a.u. and $10^{-5}$ a.u. for energies and forces, respectively). Very tight SCF convergence criterion ($10^{-10}$ a.u.) was used in all calculations. The finite-difference harmonic phonon dispersion calculations with Phonopy were carried out in identical fashion to the CRYSTAL calculations reported in the main text. In the analytical DFPT phonon dispersion calculations, we applied tight threshold for the self-consistency (tr2_ph $= 10^{-15}$) and q-point mesh of $3 \times 3 \times 3$. For the DFPT phonon dispersions, the long-range electrostatic interactions that affect the

interatomic force constants in polar compounds were taken into account using the approach developed by Gonze et al.[6]

The lattice parameters obtained from the QE PBE/GBRV-USPP (4.305 Å) and CRYSTAL PBE/TZVP (4.328 Å) calculations are in good agreement (difference of 0.5%). The electronic band gaps are also in very good agreement, both programs showing band gap of about 0.5 eV. The PBE/GBRV-USPP phonon dispersion relations calculated with Phonopy and DFPT are shown in figures 5 and 6 respectively. As can be seen from the figures, the phonon dispersion relations calculated with QE are in good agreement with each other and those calculated with CRYSTAL. Some small difference can be seen for one acoustic mode between Γ and M points, the analytical DFPT dispersion being closer to the one calculated with CRYSTAL. Similar to the GTO results, the modes between 50 and 150 $cm^{-1}$ showing the largest differences to experiment and PBE0 are also too soft when calculated with QE using a plane-wave basis set.

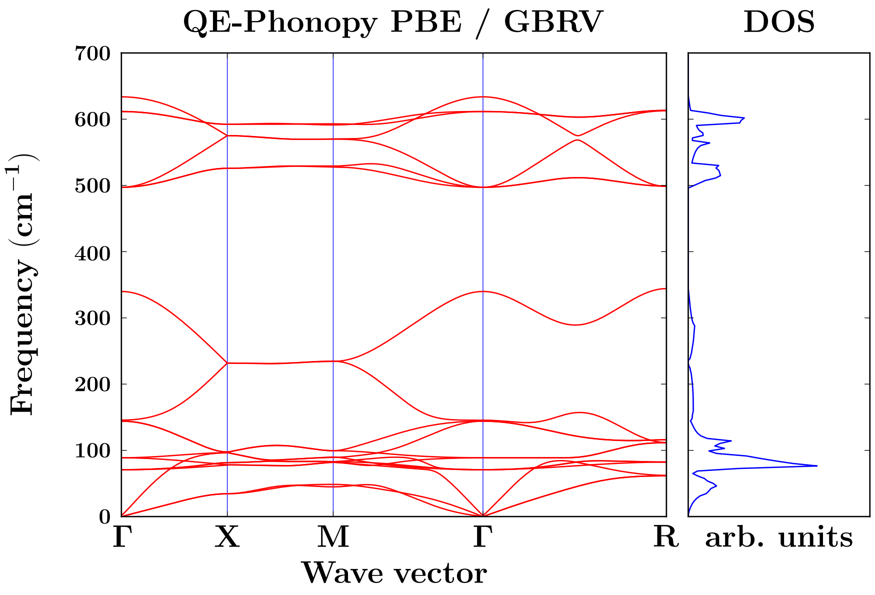


Figure 5. Phonon dispersion relations and PDOS calculated with Phonopy using Quantum Espresso as the DFT calculator (PBE/GBRV-USPP level of theory).

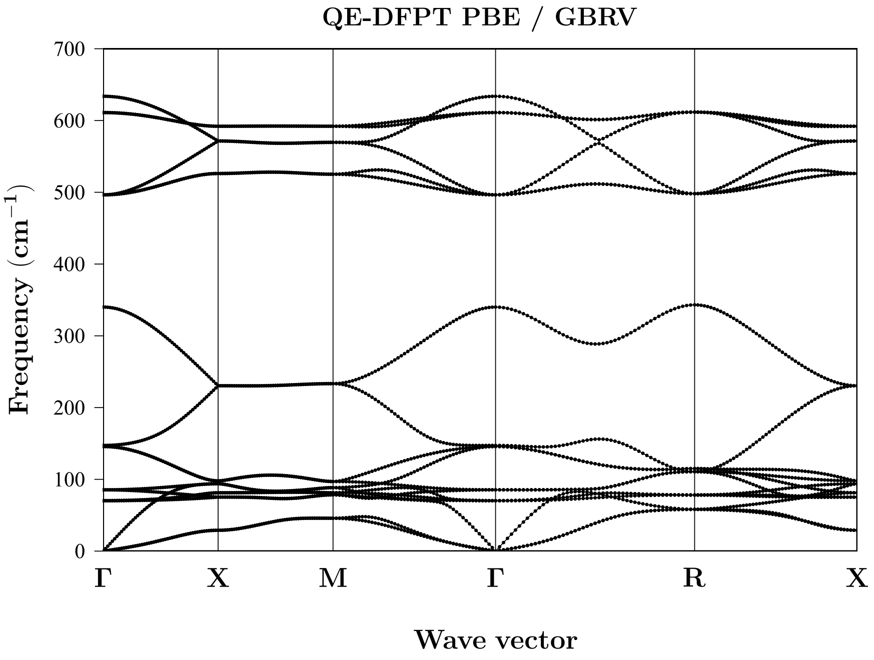


Figure 6. Phonon dispersion relations calculated with DFPT using Quantum Espresso (PBE/GBRV-USPP level of theory).

## IV. HEAT CAPACITY OF $CU_2O$

As mentioned in the main text, volumetric heat capacities obtained with both PBE and PBE0 are virtually identical, as can be seen in Figure 7. This is not surprising considering the formula from which the heat capacity is obtained,

$$C_{\mathbf{q}j} = k_B \left(\frac{\hbar\omega_{\mathbf{q}j}}{k_BT}\right)^2 \frac{\exp(\hbar\omega_{\mathbf{q}j}/k_BT)}{[\exp(\hbar\omega_{\mathbf{q}j}/k_BT)-1]^2}. \tag{1}$$

The only factors in $C_{\mathbf{q}j}$ are the phonon eigenvalues and their occupancy. When integrating over the whole frequency range, there should be practically no differences between methods when a single system is studied.

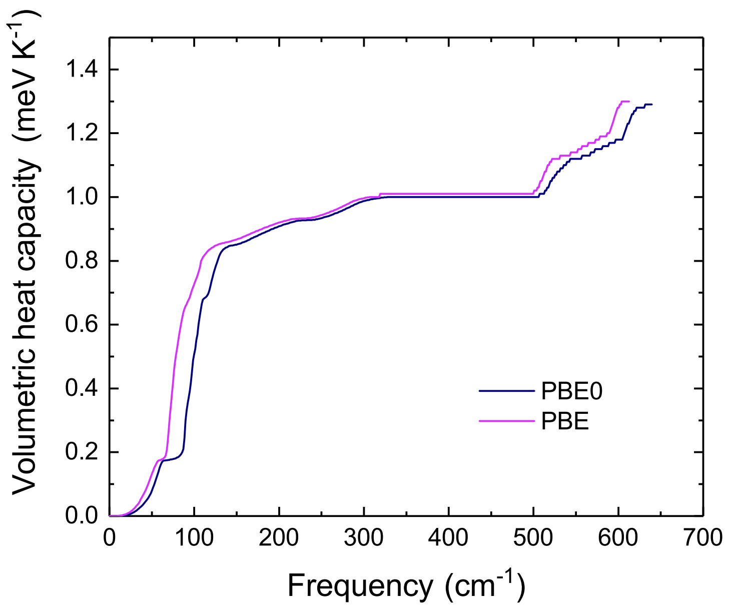


Figure 7. Volumetric heat capacity of $Cu_2O$ at the PBE/TZVP and PBE0/TZVP levels of theory.

## V. LIFETIMES AND PHONON DENSITIES

Figure 9b in the main text does not explicitly show the phonon densities of states (PDOS), but only the lifetimes. Figures 8 and 9 below contain the calculated phonon lifetimes plotted on top of PDOS (z-axis). The plot explicitly shows how in the case of PBE, the high PDOS below 4 THz (140 $cm^{-1}$) is shifted to smaller frequencies and at the same time the lifetimes become shorter in comparison to PBE0. The lifetimes shown in the figures were calculated on a $16\times16\times16$ **q**-mesh.

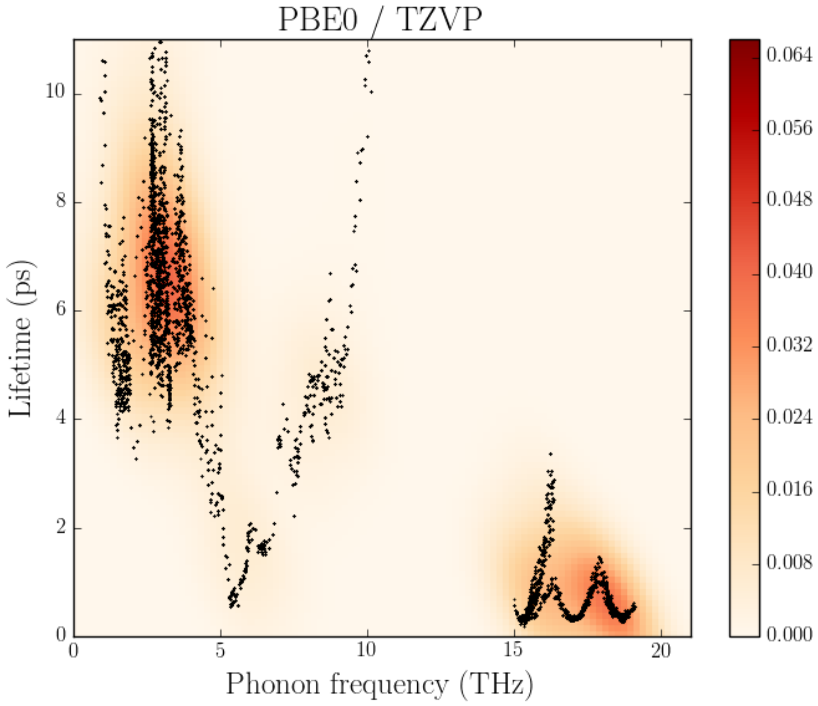


Figure 8. Phonon lifetimes plotted on top of PDOS contour plot at the PBE0/TZVP level of theory.

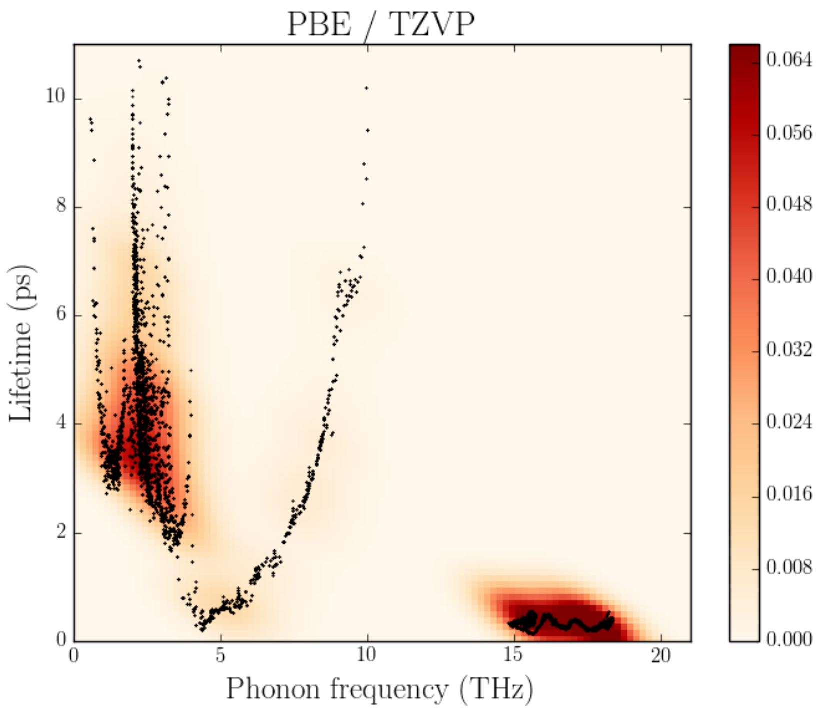


Figure 9. Phonon lifetimes plotted on top of PDOS contour plot at the PBE/TZVP level of theory.

## VI. BASIS SET INFORMATION

In periodic calculations, the Gaussian-type localized atomic basis set must be chosen carefully. Basis sets originally developed for molecular calculations contain diffuse basis functions to model the tails of wavefunction, but in periodic calculations, where the whole space is filled with basis functions, such diffuse functions are usually unnecessary and lead into numerical difficulties and/or severe degradation of performance.[7] The basis sets used in this work were obtained as follows:

**Cu**: The SVP, TZVP, and TZVPP basis sets were derived from the molecular Karlsruhe basis sets.[8] The def-SVP basis set was used as a starting point for the SVP basis set. The diffuse outermost s-exponents were increased from 0.0329 and 0.0871 to 0.14 and 0.35, respectively. The exponent of the p-type polarization function was changed from 0.155 to 0.14 and the outermost s and p functions were then combined into a single sp-type function to increase the efficiency of the CRYSTAL code. The TZVP basis set was derived from the def-TZVP basis set in an analogous way: the diffuse outermost s-exponents were increased from 0.0388 and 0.108 to 0.14 and 0.35, respectively. The exponent of the p-type polarization function was changed from 0.155 to 0.14 and the outermost s and p functions were then combined into a single sp-type function. Finally, the TZVPP level basis set was derived by replacing the outermost d-polarization function (exponent = 0.284) with two d-functions (0.380 and 0.190) and adding one f-polarization function (exponent = 2.233).

**O**: SVP, TZVP, and TZVPP basis sets were taken from a previous study.[9]

**Copper basis sets listed in CRYSTAL input format:**

```
SVP:

29 9
0 0 6 2.0 1.0
76381.348056      0.14336079896E-02
11468.777499      0.10986749865E-01
2609.4246495      0.54513652465E-01
```

```
736.75033098      0.18990128258
239.82419958      0.38581959211
82.656829252      0.29790607498
0 0 3 2.0 1.0
160.13544196     -0.11146778567
18.834177695      0.65349301031
7.7176595741      0.44770534421
0 0 3 2.0 1.0
13.710846717     -0.22870911122
2.2349895670      0.73464423031
0.87818360069     0.43273070874
0 0 1 1.0 1.0
0.35              1.00000000000
0 1 1 0.0 1.0
0.14              1.0 1.0
0 2 5 6.0 1.0
991.24075782      0.93878498798E-02
233.69376116      0.70208282458E-01
74.020930927      0.27323522220
26.664967447      0.53580792728
9.9192087478      0.34575794906
0 2 3 6.0 1.0
5.1519553926      0.34229108083
1.9638205828      0.56456592484
.71560097037      0.24078584318
0 3 4 10.0 1.0
47.335049590      0.32375547758E-01
13.161666077      0.16810218684
4.3693777244      0.38477707982
1.4132925109      0.46147880178
0 3 1 0.0 1.0
0.38878001452     0.32388873258
```

TZVP:

```
29 12
0 0 8 2.0 1.0
377518.79923      0.22811766128E-03
56589.984311      0.17688035931E-02
12878.711706      0.91993460227E-02
3645.3752143      0.37411016434E-01
1187.0072945      0.12189873737
426.46421902      0.28983900714
165.70660164      0.41531872174
65.598942707      0.21905799287
0 0 4 2.0 1.0
414.41265811     -0.24682525053E-01
128.32056039     -0.11716827406
20.622089750      0.55301315941
8.7821226045      0.52242718609
0 0 2 2.0 1.0
13.741372006      -0.22736061821
2.2431246833      0.71761210873
0 0 1 1.0 1.0
0.89370549079     1.0000000000
0 0 1 0.0 1.0
0.35              1.0000000000
0 1 1 0.0 1.0
0.14              1.0 1.0
0 2 6 6.0 1.0
2034.7596692       0.23524822298E-02
481.90468106      0.19134070751E-01
154.67482963      0.90171105278E-01
57.740576969      0.26063284735
```

```
23.099052811       0.42093485770
9.3882478591       0.24344615121
0 2 3 6.0 1.0
37.596171210       -0.28991094530E-01
5.1240690810       0.54919083831
2.0119996085       0.93793330488
0 2 1 0.0 1.0
0.73860686002      1.0000000000
0 3 4 10.0 1.0
74.129460637       0.14363216676E-01
21.359842587       0.86628177096E-01
7.4995240537       0.25631430541
2.7601394169       0.40374062368
0 3 1 0.0 1.0
0.95362061236      0.39427042447
0 3 1 0.0 1.0
0.28420862520      0.23091146816
```

TZVPP:

```
29 14
0 0 8 2.0 1.0
377518.79923       0.22811766128E-03
56589.984311       0.17688035931E-02
12878.711706       0.91993460227E-02
3645.3752143       0.37411016434E-01
1187.0072945       0.12189873737
426.46421902       0.28983900714
165.70660164       0.41531872174
65.598942707       0.21905799287
0 0 4 2.0 1.0
414.41265811      -0.24682525053E-01
```

```
128.32056039     -0.11716827406
20.622089750      0.55301315941
8.7821226045      0.52242718609
0 0 2 2.0 1.0
13.741372006      -0.22736061821
2.2431246833      0.71761210873
0 0 1 1.0 1.0
0.89370549079     1.0000000000
0 0 1 0.0 1.0
0.35              1.0000000000
0 1 1 0.0 1.0
0.14              1.0 1.0
0 2 6 6.0 1.0
2034.7596692      0.23524822298E-02
481.90468106      0.19134070751E-01
154.67482963      0.90171105278E-01
57.740576969      0.26063284735
23.099052811      0.42093485770
9.3882478591      0.24344615121
0 2 3 6.0 1.0
37.596171210     -0.28991094530E-01
5.1240690810      0.54919083831
2.0119996085      0.93793330488
0 2 1 0.0 1.0
0.73860686002     1.0000000000
0 3 4 10.0 1.0
74.129460637      0.14363216676E-01
21.359842587      0.86628177096E-01
7.4995240537      0.25631430541
2.7601394169      0.40374062368
0 3 1 0.0 1.0
0.95362061236     0.39427042447
```

```
0 3 1 0.0 1.0
0.380             1.0
0 3 1 0.0 1.0
0.190             1.0
0 4 1 0.0 1.0
2.233             1.0
```


[1] J. Sun, A. Ruzsinszky, and J. P. Perdew, Phys. Rev. Lett. **115**, 036402 (2015).

[2] K.-P. Bohnen, R. Heid, L. Pintschovius, A. Soon, and C. Stampfl, Phys. Rev. B **80**, 134304 (2009).

[3] P. Giannozzi, S. Baroni, N. Bonini, M. Calandra, R. Car, C. Cavazzoni, D. Ceresoli, G. L. Chiarotti, M. Cococcioni, I. Dabo, A. Dal Corso, S. de Gironcoli, S. Fabris, G. Fratesi, R. Gebauer, U. Gerstmann, C. Gougoussis, A. Kokalj, M. Lazzeri, L. Martin-Samos, N. Marzari, F. Mauri, R. Mazzarello, S. Paolini, A. Pasquarello, L. Paulatto, C. Sbraccia, S. Scandolo, G. Sclauzero, A. P. Seitsonen, A. Smogunov, P. Umari, and R. M. Wentzcovitch, J. Phys.: Condens. Matter **21**, 395502 (19pp) (2009).

[4] S. Baroni, S. de Gironcoli, A. Dal Corso, and P. Giannozzi, Rev. Mod. Phys. **73**, 515 (2001).

[5] K. F. Garrity, J. W. Bennett, K. M. Rabe, and D. Vanderbilt, Comput. Mater. Sci. **81**, 446 (2014).

[6] X. Gonze, J.-C. Charlier, D. Allan, and M. Teter, Phys. Rev. B **50**, 13035 (1994).

[7] K. N. Kudin and G. E. Scuseria, Phys. Rev. B **61**, 16440 (2000).

[8] F. Weigend and R. Ahlrichs, Phys. Chem. Chem. Phys. **7**, 3297 (2005).

[9] A. J. Karttunen, T. Tynell, and M. Karppinen, J. Phys. Chem. C **119**, 13105 (2015).
